# Supplementary material for: A Fully Spiking Hybrid Neural Network for Energy-Efficient Object Detection
Source: arXiv:2104.10719 source file (2021-07-24)
Supplement: Supplementary file 1 [file appendix.tex]

\section*{Appendix}

In order to do so, we consider a simple two hidden layer neural network which is updated using the STDB rule. As shown in \cite{rathi2020enabling}, the dynamics of the neuron in the output layer is described by the 

\begin{equation}
u_{i}^{t}=u_{i}^{t-1}+\sum_{j} w_{i j} o_{j} \quad
L &=-\sum_{i} y_{i} \log \left(p_{i}\right) \quad
p_{i} &=\frac{e^{u_{i}^{T}}}{\sum_{k=1}^{N} e^{u_{k}^{T}}}
\end{equation}

where $L$ is the loss function, $y$ the true output,$p$ the prediction, $T$ the total number of time steps, $u^T$ the  accumulated  membrane  potential  of  the  neuron  in  the  output  layer  from  all  time  steps,  and $N$ the number of categories in the task.

The derivative of the loss function w.r.t. to the membrane potential of the neuron in the final layer is described by $\frac{\partial L}{\partial u_{i}^{T}}=p_{i}-y_{i}$
To compute the gradient at current time step, the membrane potential at last time step $\left(u_{i}^{t-1}\right.$ in Equation $\overline{4}$ ) is considered as an input quantity. Therefore, gradient descent updates the network parameters $W_{i j}$ of the output layer as,
\begin{align}
\begin{array}{c}
W_{i j}=W_{i j}-\eta \Delta W_{i j} \\
\Delta W_{i j}=\sum_{t} \frac{\partial L}{\partial W_{i j}^{t}}=\sum_{t} \frac{\partial L}{\partial u_{i}^{T}} \frac{\partial u_{i}^{T}}{\partial W_{i j}^{t}}=\frac{\partial L}{\partial u_{i}^{T}} \sum_{t} \frac{\partial u_{i}^{T}}{\partial W_{i j}^{t}}
\end{array}
\end{align}
where $\eta$ is the learning rate, and $W_{i j}^{t}$ represents the copy of the weight used for computation at time step $t$. In the output layer the neurons do not generate a spike, and hence, the issue of non-differentiability is not encountered.

The update of the hidden layer parameters is described by,
$$
\Delta W_{i j}=\sum_{t} \frac{\partial L}{\partial W_{i j}^{t}}=\sum_{t} \frac{\partial L}{\partial o_{i}^{t}} \frac{\partial o_{i}^{t}}{\partial u_{i}^{t}} \frac{\partial u_{i}^{t}}{\partial W_{i j}^{t}}
$$
where $o_{i}^{t}$ is the thresholding function (Equation 3 whose derivative w.r.t to $u_{i}^{t}$ is zero everywhere and not defined at the time of spike. The challenge of discontinuous spiking nonlinearity is resolved by introducing a surrogate gradient which is the continuous approximation of the real gradient.
$$
\frac{\partial o_{i}^{t}}{\partial u_{i}^{t}}=\alpha e^{-\beta \Delta t}
$$
where $\alpha$ and $\beta$ are constants, $\Delta t$ is the time difference between the current time step $(t)$ and the last time step the post-neuron generated a spike $\left(t_{s}\right) .$ It is an integer value whose range is from zero to the total number of time steps $(T)$
$$
\Delta t=\left(t-t_{s}\right), 0<\Delta t<T, \Delta t \in \mathbb{Z}
$$
The values of $\alpha$ and $\beta$ are selected depending on the value of $T$. If $T$ is large $\beta$ is lowered to reduce the exponential decay so a spike can contribute towards gradients for later time steps. The value of $\alpha$ is also reduced for large $T$ because the gradient can propagate through many time steps. The gradient is summed at each time step and thus a large $\alpha$ may lead to exploding gradient.

Now, we consider a two-layer ReLU activated neural network with $m$ neurons in the hidden layer:
$$
f_{\mathbf{W}, \mathbf{a}}(\mathbf{x})=\frac{1}{\sqrt{m}} \sum_{r=1}^{m} a_{r} \sigma\left(\mathbf{w}_{r}^{\top} \mathbf{x}\right)
$$
where $\mathbf{x} \in \mathbb{R}^{d}$ is the input, $\mathbf{w}_{1}, \ldots, \mathbf{w}_{m} \in \mathbb{R}^{d}$ are weight vectors in the first layer, $a_{1}, \ldots, a_{m} \in \mathbb{R}$ are weights in the second layer. For convenience we denote $\mathbf{W}=\left(\mathbf{w}_{1}, \ldots, \mathbf{w}_{m}\right) \in \mathbb{R}^{d \times m}$ and $\mathbf{a}=\left(a_{1}, \ldots, a_{m}\right)^{\top} \in \mathbb{R}^{m}$
We are given $n$ input-label samples $S=\left\{\left(\mathbf{x}_{i}, y_{i}\right)\right\}_{i=1}^{n}$ drawn i.i.d. from an underlying data distribution $\mathcal{D}$ over $\mathbb{R}^{d} \times \mathbb{R} .$ We denote $\mathbf{X}=\left(\mathbf{x}_{1}, \ldots, \mathbf{x}_{n}\right) \in \mathbb{R}^{d \times n}$ and $\mathbf{y}=\left(y_{1}, \ldots, y_{n}\right)^{\top} \in \mathbb{R}^{n} .$ For simplicity, we assume
that for $(\mathrm{x}, y)$ sampled from $\mathcal{D},$ we have $\|\mathrm{x}\|_{2}=1$ and $|y| \leq 1$ We train the neural network by randomly initialized gradient descent $(G D)$ on the quadratic loss over data $S .$ In particular, we first initialize the parameters randomly:
$$
\mathbf{w}_{r}(0) \sim \mathcal{N}\left(\mathbf{0}, \kappa^{2} \mathbf{I}\right), a_{r} \sim \text { unif }(\{-1,1\}), \quad \forall r \in[m]
$$
where $0<\kappa \leq 1$ controls the magnitude of initialization, and all randomnesses are independent. We then fix the second layer a and optimize the first layer $\mathbf{W}$ through GD on the following objective function:
$$
\Phi(\mathbf{W})=\frac{1}{2} \sum_{i=1}^{n}\left(y_{i}-f_{\mathbf{W}, \mathbf{a}}\left(\mathbf{x}_{i}\right)\right)^{2}
$$
